# Supplementary material for: ASASSN-18aan: An Eclipsing SU UMa-type Cataclysmic Variable with a 3.6-hour Orbital Period and a Late G-type Secondary Star
Source: arXiv:2102.04104 ancillary file (2021-02-09)
Supplement: Supplementary file 1 [file si.pdf]

**Table E1.** List of eclipses in ASASSN-18aan.

| Number | Time* | ingress† | egress† | Radius‡ | error1§ | error2‖ | Exponent | error1§ | error2‖ | Filter# |
|---|---|---|---|---|---|---|---|---|---|---|
| 1 | 57.393293 | -0.11 | 0.11 | 0.446 | 0.012 | -0.012 | -0.538 | 0.019 | -0.018 | C |
| 2 | 57.542749 | -0.10 | 0.10 | 0.353 | 0.009 | -0.010 | -0.384 | 0.031 | -0.025 | C |
| 8 | 58.439485 | -0.10 | 0.10 | 0.411 | 0.013 | -0.012 | -0.587 | 0.022 | -0.019 | C |
| 9a | 58.588941 | -0.10 | 0.10 | 0.389 | 0.018 | -0.015 | -0.569 | 0.030 | -0.027 | C |
| 9b | 58.588941 | -0.08 | 0.08 | 0.279 | 0.009 | -0.010 | -0.486 | 0.029 | -0.026 | B |
| 10 | 58.738397 | -0.10 | 0.10 | 0.457 | 0.017 | -0.021 | -0.586 | 0.025 | -0.022 | C |
| 14 | 59.336221 | -0.08 | 0.08 | 0.300 | 0.013 | -0.011 | -0.564 | 0.032 | -0.028 | C |
| 15 | 59.485677 | -0.08 | 0.08 | 0.288 | 0.016 | -0.014 | -0.511 | 0.046 | -0.039 | C |
| 21 | 60.382413 | -0.09 | 0.09 | 0.378 | 0.012 | -0.011 | -0.429 | 0.032 | -0.031 | C |
| 22 | 60.531869 | -0.09 | 0.09 | 0.364 | 0.016 | -0.013 | -0.465 | 0.032 | -0.030 | C |
| 25 | 60.980237 | -0.08 | 0.08 | 0.282 | 0.014 | -0.013 | -0.553 | 0.042 | -0.034 | V |
| 27 | 61.279149 | -0.08 | 0.08 | 0.291 | 0.013 | -0.012 | -0.560 | 0.031 | -0.031 | C |
| 28a | 61.428605 | -0.07 | 0.07 | 0.250 | 0.011 | -0.010 | -0.585 | 0.036 | -0.036 | B |
| 28b | 61.428605 | -0.07 | 0.07 | 0.267 | 0.013 | -0.011 | -0.510 | 0.038 | -0.039 | V |
| 31 | 61.876973 | -0.07 | 0.07 | 0.276 | 0.011 | -0.011 | -0.330 | 0.056 | -0.045 | V |
| 38a | 62.923165 | -0.08 | 0.08 | 0.362 | 0.015 | -0.014 | -0.573 | 0.026 | -0.027 | g |
| 38b | 62.923165 | -0.09 | 0.09 | 0.419 | 0.015 | -0.013 | -0.363 | 0.036 | -0.035 | Ic |
| 38c | 62.923165 | -0.08 | 0.08 | 0.440 | 0.017 | -0.015 | -0.537 | 0.025 | -0.026 | Rc |
| 39a | 63.072621 | -0.10 | 0.10 | 0.403 | 0.010 | -0.010 | -0.396 | 0.025 | -0.021 | Ic |
| 39b | 63.072621 | -0.08 | 0.08 | 0.340 | 0.012 | -0.011 | -0.549 | 0.027 | -0.024 | V |
| 39c | 63.072621 | -0.08 | 0.08 | 0.340 | 0.010 | -0.011 | -0.454 | 0.027 | -0.029 | C |
| 39d | 63.072621 | -0.09 | 0.09 | 0.402 | 0.011 | -0.007 | -0.384 | 0.023 | -0.029 | i |
| 39e | 63.072621 | -0.09 | 0.09 | 0.362 | 0.008 | -0.009 | -0.577 | 0.020 | -0.018 | r |
| 40 | 63.222077 | -0.09 | 0.09 | 0.405 | 0.007 | -0.009 | -0.604 | 0.012 | -0.011 | C |
| 41 | 63.371533 | -0.08 | 0.08 | 0.305 | 0.019 | -0.014 | -0.568 | 0.038 | -0.041 | C |
| 42 | 63.520989 | -0.07 | 0.07 | 0.308 | 0.013 | -0.011 | -0.608 | 0.033 | -0.028 | C |
| 52a | 65.015549 | -0.06 | 0.06 | 0.237 | 0.010 | -0.009 | -0.443 | 0.051 | -0.045 | g |
| 52b | 65.015549 | -0.09 | 0.09 | 0.352 | 0.024 | -0.018 | -0.454 | 0.054 | -0.040 | Ic |
| 52c | 65.015549 | -0.07 | 0.07 | 0.301 | 0.017 | -0.013 | -0.423 | 0.046 | -0.048 | Rc |
| 52d | 65.015549 | -0.07 | 0.07 | 0.303 | 0.032 | -0.019 | -0.613 | 0.052 | -0.053 | V |
| 53 | 65.165005 | -0.07 | 0.07 | 0.266 | 0.021 | -0.017 | -0.453 | 0.078 | -0.070 | V |
| 54 | 65.314461 | -0.08 | 0.08 | 0.361 | 0.021 | -0.017 | -0.560 | 0.036 | -0.032 | C |
| 58 | 65.912285 | -0.09 | 0.09 | 0.355 | 0.018 | -0.018 | -0.491 | 0.040 | -0.034 | Ic |
| 65a | 66.958477 | -0.08 | 0.08 | 0.310 | 0.011 | -0.012 | -0.532 | 0.031 | -0.027 | Ic |
| 65b | 66.958477 | -0.07 | 0.07 | 0.268 | 0.017 | -0.013 | -0.433 | 0.057 | -0.058 | Rc |
| 65c | 66.958477 | -0.06 | 0.06 | 0.200 | 0.031 | -0.038 | -0.425 | 0.372 | -0.147 | V |
| 68a | 67.406845 | -0.07 | 0.07 | 0.279 | 0.020 | -0.025 | -0.287 | 0.139 | -0.099 | Ic |
| 68b | 67.406845 | -0.06 | 0.06 | 0.214 | 0.021 | -0.019 | -0.445 | 0.109 | -0.090 | V |
| 72a | 68.004669 | -0.09 | 0.09 | 0.428 | 0.017 | -0.013 | -0.563 | 0.024 | -0.026 | Ic |
| 72b | 68.004669 | -0.07 | 0.07 | 0.294 | 0.011 | -0.012 | -0.603 | 0.033 | -0.026 | g |
| 72c | 68.004669 | -0.08 | 0.08 | 0.306 | 0.013 | -0.013 | -0.403 | 0.052 | -0.035 | Rc |
| 81a | 69.349773 | -0.04 | 0.04 | 0.120 | 0.005 | -0.002 | 0.142 | 0.106 | -0.153 | B |
| 81b | 69.349773 | -0.07 | 0.07 | 0.316 | 0.031 | -0.025 | -0.706 | 0.046 | -0.043 | Rc |
| 135 | 77.420397 | -0.05 | 0.05 | 0.144 | 0.004 | -0.005 | -0.090 | 0.129 | -0.083 | C |
| 180 | 84.145917 | -0.05 | 0.05 | 0.138 | 0.011 | -0.006 | 0.480 | 0.385 | -0.337 | C |
| 186 | 85.042653 | -0.05 | 0.05 | 0.151 | 0.005 | -0.005 | -0.343 | 0.097 | -0.079 | C |
| 189 | 85.491021 | -0.04 | 0.04 | 0.100 | 0.001 | -0.006 | 0.124 | 0.234 | -0.076 | C |
| 190 | 85.640477 | -0.04 | 0.04 | 0.128 | 0.010 | -0.009 | -0.627 | 0.101 | -0.092 | C |

*BJD−2458400. †In units of orbital phase. ‡In units of the binary separation.

§Upper 95% credible interval. ‖Lower 95% credible interval. #Ic includes both the I and Ic passband.

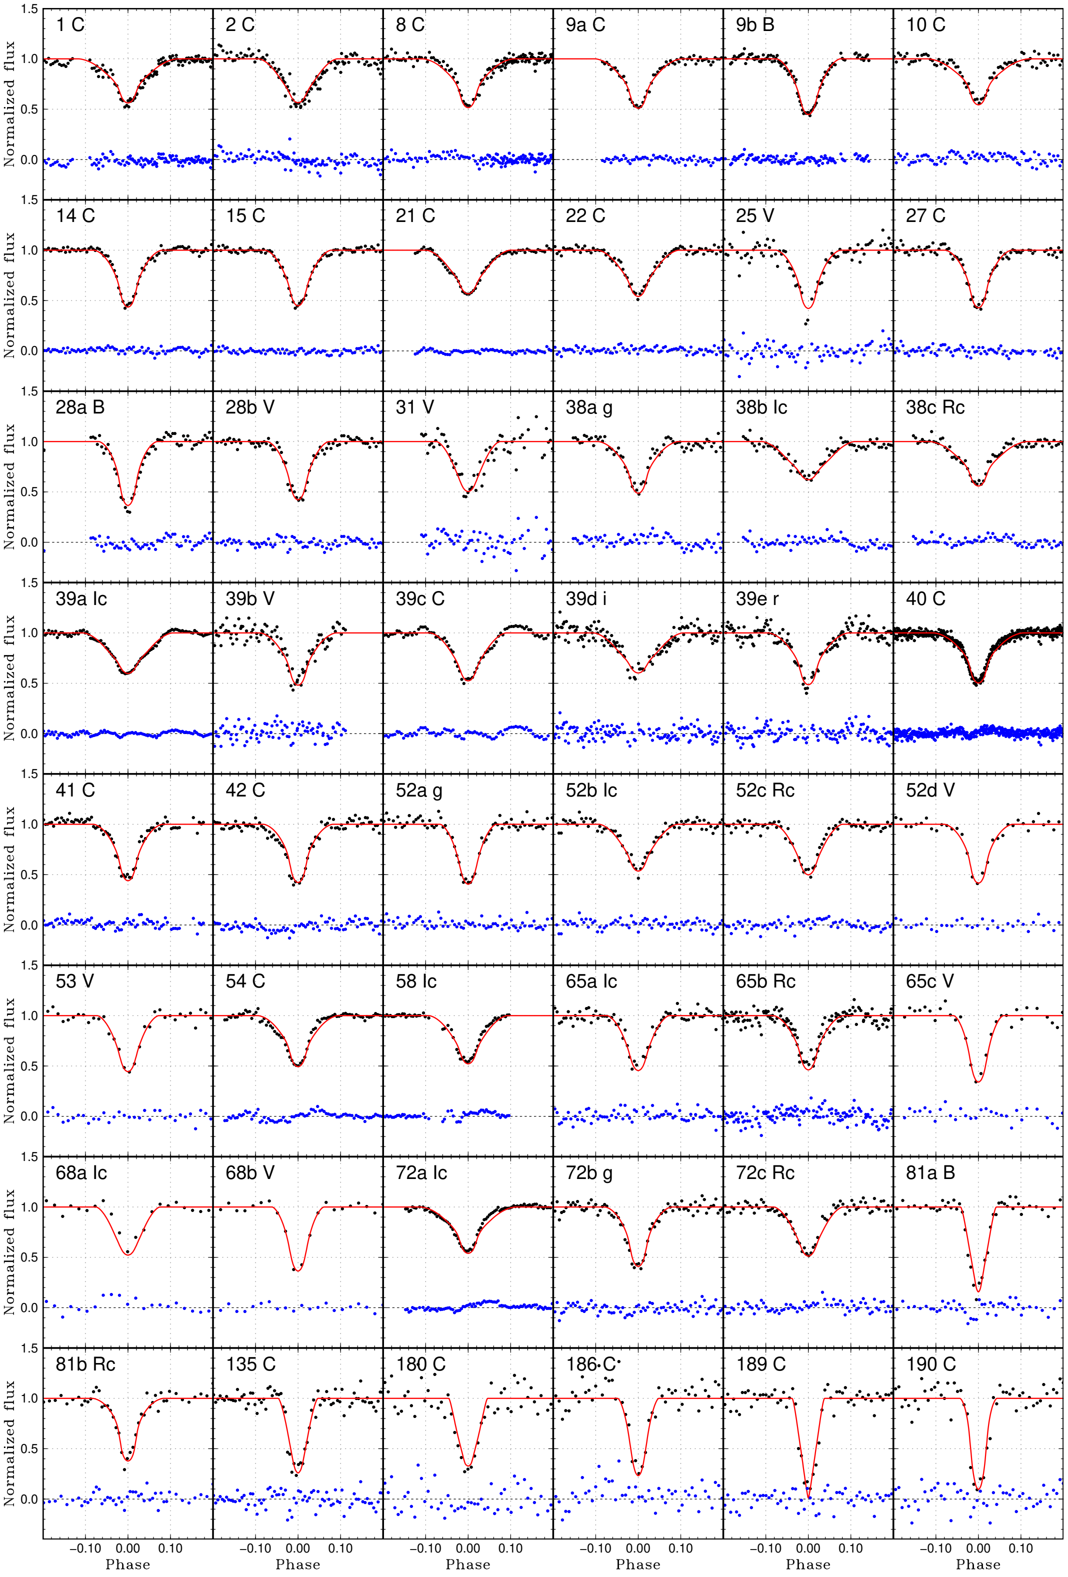


**Fig. E1.** Results of Eclipse modelings. Each label represents the eclipse number and filter, corresponding with in table E1. Each horizontal and vertical axes represent orbital phase with a range of -0.2–0.2 and Normalized flux with a range of -0.4–1.5, respectively. Dashed lines represent 0 level. Black points and red solid lines represent normalized flux and model light curves made from estimated parameters, respectively. Lower blue points represent residuals. Ic includes both the I and Ic passband.

**Table E2.** Log of observations of the superoutburst of ASASSN-18aan.

| Start* | End* | mag† | error‡ | $N$§ | obs‖ | sys# |
|---|---|---|---|---|---|---|
| 57.3510 | 57.6103 | 8.608 | 0.010 | 182 | Van | CV |
| 57.3794 | 57.6019 | 8.607 | 0.007 | 310 | Trt | C |
| 57.6547 | 57.6947 | 8.844 | 0.029 | 95 | LPA | V |
| 57.6981 | 57.7341 | 8.660 | 0.033 | 42 | LPA | B |
| 57.7381 | 57.7744 | 8.729 | 0.055 | 11 | LPA | I |
| 58.3357 | 58.5876 | 8.658 | 0.007 | 355 | Trt | C |
| 58.4407 | 58.6073 | 8.684 | 0.008 | 359 | Shu | B |
| 58.4425 | 58.5573 | 8.729 | 0.109 | 3 | Shu | V |
| 58.4432 | 58.5577 | 8.805 | 0.094 | 3 | Shu | Rc |
| 58.4440 | 58.5582 | 8.855 | 0.095 | 3 | Shu | Ic |
| 58.5734 | 58.7647 | 8.732 | 0.008 | 257 | DFS | CV |
| 59.2820 | 59.5622 | 8.635 | 0.012 | 375 | DFS | CV |
| 60.0453 | 60.1843 | 8.616 | 0.021 | 121 | Ioh | C |
| 60.2817 | 60.5623 | 8.655 | 0.007 | 298 | DFS | CV |
| 60.3608 | 60.4550 | 8.655 | 0.009 | 114 | Van | CV |
| 60.5850 | 60.6069 | 8.796 | 0.014 | 55 | LPA | V |
| 60.6091 | 60.6548 | 8.809 | 0.020 | 55 | LPA | B |
| 60.6571 | 60.6648 | 8.660 | 0.045 | 18 | LPA | I |
| 60.8946 | 61.0596 | 8.620 | 0.016 | 211 | KU1 | V |
| 60.9267 | 61.2862 | 8.730 | 0.025 | 291 | Ioh | C |
| 61.0545 | 61.1223 | 8.647 | 0.060 | 14 | MIT | g |
| 61.0545 | 61.1231 | 8.709 | 0.046 | 27 | MIT | Ic |
| 61.0553 | 61.1223 | 8.723 | 0.033 | 16 | MIT | Rc |
| 61.2238 | 61.4088 | 8.559 | 0.017 | 222 | Trt | CV |
| 61.3398 | 61.5894 | 8.619 | 0.020 | 217 | Shu | V |
| 61.3429 | 61.4922 | 8.570 | 0.029 | 130 | Shu | B |
| 61.3650 | 61.3650 | 8.473 | – | 1 | TRT | CV |
| 61.4808 | 61.5917 | 9.070 | 0.039 | 24 | Shu | Ic |
| 61.4811 | 61.4811 | 8.433 | – | 1 | Shu | Rc |
| 61.5922 | 61.6185 | 8.714 | 0.016 | 25 | LPA | V |
| 61.6222 | 61.6619 | 8.409 | 0.027 | 25 | LPA | B |
| 61.6651 | 61.6805 | 8.447 | 0.040 | 15 | LPA | I |
| 61.8577 | 62.0209 | 8.541 | 0.022 | 148 | KU1 | V |
| 61.8769 | 62.1490 | 8.460 | 0.012 | 224 | Ioh | C |
| 62.0786 | 62.1216 | 8.487 | 0.030 | 21 | OKU | V |
| 62.8973 | 62.9594 | 8.586 | 0.024 | 79 | MIT | g |
| 62.8973 | 62.9594 | 8.630 | 0.022 | 78 | MIT | Rc |
| 62.8973 | 62.9594 | 8.645 | 0.020 | 79 | MIT | Ic |

*BJD−2458400.
†Mean magnitude.
‡1-$\sigma$ of the mean magnitude.
§Number of observations.
‖Observer's code: Van (T. Vanmunster), Trt (T. Tordai), Shu (S. Shugarov team), Ioh (H. Itoh), KU1 (Kyoto U., campus obs.), MIT (MITSuME, Tokyo Institute of Technology), OKU (Osaka Kyoiku U.) and AAVSO collaboration.
#Filter. "C" means no filter (clear).

**Table E2.** Log of observations of the superoutburst of ASASSN-18aan (contiuned).

| Start* | End* | mag† | error‡ | $N$§ | obs‖ | sys# |
|---|---|---|---|---|---|---|
| 62.9172 | 63.1988 | 8.601 | 0.011 | 148 | OKU | V |
| 62.9457 | 63.3178 | 8.522 | 0.014 | 212 | Ioh | V |
| 62.9459 | 63.0977 | 8.611 | 0.011 | 201 | Mzm | C |
| 62.9466 | 63.3255 | 8.562 | 0.016 | 215 | Ioh | Ic |
| 62.9611 | 63.1581 | 8.640 | 0.007 | 318 | hho | I |
| 62.9611 | 63.1900 | 8.644 | 0.009 | 271 | KU1 | V |
| 62.9654 | 62.9745 | 8.638 | 0.012 | 24 | SCR | z |
| 62.9654 | 63.2715 | 8.580 | 0.007 | 498 | SCR | r |
| 62.9658 | 63.2670 | 8.594 | 0.007 | 424 | SCR | i |
| 63.1395 | 63.2993 | 8.590 | 0.005 | 1180 | Kso | C |
| 63.3045 | 63.6139 | 8.603 | 0.010 | 412 | Trt | CV |
| 64.8959 | 65.1930 | 8.675 | 0.015 | 157 | OKU | V |
| 64.9792 | 65.0620 | 8.698 | 0.024 | 98 | MIT | g |
| 64.9792 | 65.0620 | 8.707 | 0.019 | 102 | MIT | Rc |
| 64.9792 | 65.0620 | 8.716 | 0.018 | 101 | MIT | Ic |
| 65.2629 | 65.4070 | 8.782 | 0.010 | 186 | Van | CV |
| 65.8709 | 66.1397 | 8.837 | 0.009 | 339 | KU1 | V |
| 65.8717 | 65.9238 | 8.906 | 0.021 | 74 | hho | I |
| 66.0344 | 66.0400 | 8.850 | 0.021 | 3 | MIT | Rc |
| 66.0575 | 66.1801 | 8.779 | 0.030 | 66 | OKU | V |
| 66.3667 | 66.4863 | 8.768 | 0.006 | 152 | Van | CV |
| 66.8849 | 67.0692 | 8.848 | 0.025 | 83 | OKU | V |
| 66.9129 | 67.0519 | 8.863 | 0.010 | 133 | SCR | z |
| 66.9129 | 67.0519 | 8.871 | 0.015 | 113 | SCR | Ic |
| 66.9165 | 67.0519 | 8.842 | 0.012 | 113 | SCR | r |
| 66.9191 | 67.0028 | 8.883 | 0.019 | 87 | MIT | g |
| 66.9191 | 67.0028 | 8.885 | 0.018 | 104 | MIT | Rc |
| 66.9191 | 67.0028 | 8.887 | 0.018 | 103 | MIT | Ic |
| 67.2940 | 67.4824 | 8.871 | 0.024 | 67 | DPV | V |
| 67.2954 | 67.4781 | 8.863 | 0.017 | 65 | DPV | I |
| 67.8512 | 68.1778 | 9.235 | 0.041 | 162 | Ioh | V |
| 67.8531 | 68.1787 | 9.194 | 0.038 | 164 | Ioh | Ic |
| 67.8915 | 68.0625 | 8.979 | 0.018 | 75 | OKU | V |
| 67.8952 | 68.3089 | 9.076 | 0.012 | 289 | KU1 | V |
| 67.9583 | 68.0418 | 8.928 | 0.012 | 104 | MIT | Ic |
| 67.9583 | 68.0418 | 8.959 | 0.014 | 103 | MIT | Rc |
| 67.9583 | 68.0418 | 9.013 | 0.019 | 105 | MIT | g |
| 67.9799 | 68.0676 | 8.975 | 0.010 | 141 | hho | I |

*BJD−2458400.
†Mean magnitude.
‡1-$\sigma$ of the mean magnitude.
§Number of observations.
‖Observer's code: OKU (Osaka Kyoiku U.), Ioh (H. Itoh), Mzm (M. Mizutani), hho (Kanata, Hiroshima U.), KU1 (Kyoto U., campus obs.), SCR (SaCRA, Saitama U.), Kso (Kiso, The U. of Tokyo), Trt (T. Tordai), MIT (MITSuME, Tokyo Institute of Technology), Van (T. Vanmunster), DPV (P. Dubovsky).
#Filter. "C" means no filter (clear).

**Table E2.** Log of observations of the superoutburst of ASASSN-18aan (contiuned).

| Start* | End* | mag† | error‡ | $N$§ | obs‖ | sys# |
|---|---|---|---|---|---|---|
| 69.2193 | 69.3779 | 9.264 | 0.020 | 102 | Shu | Rc |
| 69.2256 | 69.3758 | 9.277 | 0.036 | 88 | Shu | B |
| 69.2289 | 69.3764 | 9.116 | 0.007 | 52 | Shu | V |
| 69.2300 | 69.3774 | 9.189 | 0.008 | 50 | Shu | Ic |
| 69.9737 | 70.0830 | 9.173 | 0.015 | 55 | OKU | V |
| 70.0456 | 70.2674 | 9.267 | 0.028 | 32 | SCR | r |
| 70.0456 | 70.2689 | 9.202 | 0.014 | 64 | SCR | i |
| 70.0464 | 70.2674 | 9.381 | 0.050 | 16 | SCR | z |
| 70.3355 | 70.3568 | 9.319 | 0.005 | 29 | VMT | CV |
| 70.8611 | 70.9686 | 9.484 | 0.015 | 147 | KU1 | V |
| 71.0791 | 71.1763 | 9.541 | 0.036 | 48 | OKU | V |
| 71.1042 | 71.2073 | 9.378 | 0.017 | 108 | hho | I |
| 71.3282 | 71.6270 | 9.719 | 0.015 | 168 | DPV | C |
| 71.3931 | 71.5756 | 9.633 | 0.010 | 47 | Shu | V |
| 71.3948 | 71.5746 | 9.898 | 0.030 | 87 | Shu | B |
| 71.3964 | 71.5763 | 9.611 | 0.011 | 44 | Shu | Rc |
| 71.3973 | 71.6143 | 9.696 | 0.014 | 111 | Shu | Ic |
| 71.8748 | 72.1693 | 9.547 | 0.013 | 101 | SCR | z |
| 71.8748 | 72.2087 | 9.743 | 0.030 | 57 | SCR | r |
| 71.8763 | 72.0149 | 9.749 | 0.047 | 52 | KU1 | V |
| 71.8770 | 72.2190 | 9.581 | 0.019 | 67 | SCR | i |
| 72.0019 | 72.0756 | 9.611 | 0.018 | 74 | hho | I |
| 72.2934 | 72.3349 | 9.717 | 0.021 | 53 | Van | CV |
| 72.9986 | 73.1475 | 9.958 | 0.016 | 61 | ISH | Ic |
| 73.0240 | 73.1538 | 9.898 | 0.009 | 77 | ISH | Rc |
| 73.0248 | 73.1601 | 9.901 | 0.014 | 61 | ISH | g |
| 73.0771 | 73.1267 | 9.933 | 0.068 | 6 | KU1 | V |
| 74.8706 | 75.0097 | 9.543 | 0.015 | 141 | KU1 | C |
| 74.9344 | 74.9857 | 9.403 | 0.028 | 18 | OKU | V |
| 76.0477 | 76.2159 | 9.077 | 0.029 | 33 | SCR | r |
| 76.0484 | 76.2159 | 9.074 | 0.014 | 81 | SCR | z |
| 76.0484 | 76.2195 | 9.105 | 0.028 | 36 | SCR | i |
| 76.0738 | 76.2328 | 9.075 | 0.013 | 193 | Ioh | C |
| 76.8842 | 77.0956 | 9.710 | 0.019 | 100 | OKU | V |
| 76.9947 | 77.2536 | 9.836 | 0.013 | 267 | KU1 | C |
| 77.3506 | 77.5198 | 9.708 | 0.010 | 214 | Van | CV |
| 77.8567 | 78.1566 | 10.030 | 0.015 | 215 | KU1 | C |
| 77.8856 | 78.0603 | 9.923 | 0.024 | 65 | OKU | V |

*BJD−2458400.

†Mean magnitude.

‡1-$\sigma$ of the mean magnitude.

§Number of observations.

‖Observer's code: Shu (S. Shugarov team), OKU (Osaka Kyoiku U.), SCR (SaCRA, Saitama U.), KU1 (Kyoto U., campus obs.), hho (Kanata, Hiroshima U.), DPV (P. Dubovsky), Van (T. Vanmunster), ISH (Murikabushi, Ishigakijima Astronomical Obs.), Ioh (H. Itoh) and AAVSO collaboration.

#Filter. "C" means no filter (clear).

**Table E2.** Log of observations of the superoutburst of ASASSN-18aan (contiuned).

| Start* | End* | mag† | error‡ | $N$§ | obs‖ | sys# |
|---|---|---|---|---|---|---|
| 78.4316 | 78.5401 | 9.874 | 0.010 | 138 | Van | CV |
| 79.3126 | 79.4889 | 9.913 | 0.010 | 148 | Van | CV |
| 79.4349 | 79.4603 | 10.001 | 0.066 | 5 | Shu | Rc |
| 79.4364 | 79.4411 | 10.079 | 0.067 | 5 | Shu | Ic |
| 79.4437 | 79.5473 | 9.917 | 0.022 | 53 | Shu | CR |
| 79.8753 | 80.0083 | 10.096 | 0.011 | 82 | hho | V |
| 79.8881 | 80.1392 | 10.104 | 0.019 | 82 | OKU | V |
| 79.9062 | 80.0169 | 10.056 | 0.012 | 69 | hho | I |
| 79.9145 | 80.0693 | 10.138 | 0.016 | 78 | KU1 | C |
| 81.0275 | 81.2586 | 9.789 | 0.020 | 199 | Ioh | C |
| 81.3073 | 81.4665 | 10.108 | 0.015 | 115 | Trt | CV |
| 81.8692 | 82.2522 | 9.929 | 0.012 | 326 | Ioh | C |
| 81.8813 | 82.1980 | 10.187 | 0.017 | 56 | KU1 | C |
| 82.2841 | 82.4566 | 10.006 | 0.008 | 232 | DFS | CV |
| 82.8670 | 83.1467 | 9.961 | 0.027 | 239 | Ioh | C |
| 83.9116 | 84.1965 | 9.213 | 0.013 | 230 | Ioh | C |
| 84.2604 | 84.2880 | 9.586 | 0.055 | 12 | KU1 | C |
| 84.3545 | 84.3839 | 9.347 | 0.015 | 19 | Shu | Rc |
| 84.8825 | 85.1954 | 9.321 | 0.018 | 267 | Ioh | C |
| 85.4540 | 85.5824 | 9.654 | 0.015 | 127 | Van | CV |
| 85.5785 | 85.6881 | 9.760 | 0.016 | 95 | SGE | CV |
| 85.9056 | 86.1781 | 9.789 | 0.015 | 234 | Ioh | C |
| 85.9619 | 86.1269 | 9.766 | 0.011 | 219 | Mzm | C |
| 86.5793 | 86.8144 | 10.037 | 0.009 | 200 | SGE | CV |
| 86.8743 | 87.1321 | 10.170 | 0.021 | 211 | Ioh | C |
| 87.2036 | 87.3739 | 10.037 | 0.015 | 122 | Trt | CV |
| 87.3101 | 87.5723 | 10.043 | 0.011 | 187 | IMi | CV |
| 87.3197 | 87.4469 | 10.061 | 0.017 | 81 | Van | CV |
| 87.8566 | 88.2053 | 10.294 | 0.045 | 282 | Ioh | C |
| 88.8649 | 89.1512 | 9.879 | 0.018 | 233 | Ioh | C |
| 88.8927 | 88.9950 | 10.196 | 0.033 | 23 | OKU | V |
| 89.8738 | 90.0388 | 10.157 | 0.023 | 79 | OKU | V |
| 90.8688 | 91.0425 | 10.118 | 0.020 | 82 | OKU | V |
| 90.9691 | 91.0834 | 10.079 | 0.015 | 42 | hho | V |
| 90.9701 | 91.0844 | 10.084 | 0.014 | 53 | hho | I |
| 91.8696 | 91.9758 | 10.047 | 0.027 | 31 | OKU | V |
| 93.0349 | 93.1177 | 10.176 | 0.039 | 40 | OKU | V |
| 94.8834 | 95.1321 | 9.992 | 0.018 | 209 | Ioh | C |

*BJD−2458400.

†Mean magnitude.

‡1-$\sigma$ of the mean magnitude.

§Number of observations.

‖Observer's code: Van (T. Vanmunster), Shu (S. Shugarov team), hho (Kanata, Hiroshima U.), OKU (Osaka Kyoiku U.), KU1 (Kyoto U., campus obs.), Ioh (H. Itoh), Trt (T. Tordai), SGE (G. Stone), Mzm (M. Mizutani), IMi (I. Miller) and AAVSO collaboration.

#Filter. "C" means no filter (clear).

**Table E2.** Log of observations of the superoutburst of ASASSN-18aan (contiuned).

| Start* | End* | mag† | error‡ | $N$§ | obs‖ | sys# |
|---|---|---|---|---|---|---|
| 94.9128 | 95.0256 | 10.154 | 0.026 | 58 | OKU | V |
| 95.9769 | 96.0861 | 10.164 | 0.026 | 58 | OKU | V |
| 96.8786 | 97.1057 | 10.198 | 0.016 | 100 | OKU | V |
| 96.8985 | 97.0477 | 10.154 | 0.012 | 65 | hho | V |
| 96.8995 | 97.0466 | 10.125 | 0.011 | 66 | hho | I |
| 97.8760 | 98.1022 | 10.202 | 0.023 | 97 | OKU | V |
| 97.8860 | 98.2072 | 10.216 | 0.043 | 269 | Ioh | C |
| 97.8902 | 98.0435 | 10.139 | 0.012 | 59 | hho | I |
| 97.9076 | 98.0343 | 10.068 | 0.017 | 29 | hho | V |
| 97.9546 | 98.0084 | 10.267 | 0.021 | 69 | KU1 | C |
| 98.8948 | 98.9973 | 10.056 | 0.032 | 23 | hho | V |
| 98.8959 | 98.9962 | 10.132 | 0.028 | 20 | hho | I |
| 99.8936 | 100.0971 | 10.122 | 0.019 | 98 | OKU | V |
| 99.9081 | 99.9941 | 10.206 | 0.029 | 25 | hho | V |
| 99.9091 | 99.9971 | 10.178 | 0.021 | 39 | hho | I |
| 101.9194 | 102.0771 | 10.308 | 0.036 | 24 | OKU | V |
| 101.9860 | 102.0715 | 10.347 | 0.035 | 39 | KU1 | C |
| 102.8834 | 103.0070 | 10.269 | 0.020 | 100 | KU1 | C |
| 102.8849 | 103.0210 | 10.152 | 0.021 | 74 | OKU | V |
| 103.8841 | 103.9940 | 10.086 | 0.024 | 40 | OKU | V |
| 104.8813 | 105.0536 | 10.050 | 0.033 | 49 | OKU | V |
| 104.8891 | 104.9755 | 10.123 | 0.016 | 85 | KU1 | C |
| 105.8845 | 106.0618 | 10.127 | 0.023 | 88 | OKU | V |
| 105.9418 | 106.1452 | 10.239 | 0.016 | 155 | KU1 | C |
| 106.9133 | 107.0655 | 9.960 | 0.033 | 39 | OKU | V |
| 107.9044 | 108.0691 | 10.196 | 0.023 | 87 | OKU | V |
| 108.0149 | 108.0902 | 10.175 | 0.038 | 25 | ISH | g |
| 108.0165 | 108.0910 | 10.128 | 0.014 | 65 | ISH | Rc |
| 108.0165 | 108.0926 | 10.128 | 0.015 | 43 | ISH | Ic |
| 109.8861 | 110.0549 | 10.187 | 0.025 | 68 | OKU | V |
| 109.8896 | 110.0741 | 10.222 | 0.054 | 168 | Ioh | C |
| 110.8922 | 111.0661 | 11.095 | 0.067 | 146 | Ioh | C |
| 110.9194 | 111.0231 | 10.208 | 0.017 | 141 | KU1 | C |
| 110.9289 | 111.0291 | 10.174 | 0.031 | 52 | OKU | V |
| 111.9925 | 112.0087 | 10.377 | 0.073 | 10 | OKU | V |
| 113.0248 | 113.0606 | 10.215 | 0.065 | 19 | OKU | V |
| 113.0927 | 113.1358 | 10.144 | 0.029 | 51 | KU1 | C |
| 113.8813 | 113.9798 | 10.200 | 0.029 | 56 | OKU | V |
| 113.8835 | 113.9719 | 10.189 | 0.018 | 95 | KU1 | C |
| 116.9023 | 117.0270 | 10.146 | 0.019 | 53 | hho | V |
| 116.9034 | 117.0260 | 10.116 | 0.014 | 61 | hho | I |

*BJD−2458400.

†Mean magnitude.

‡1-$\sigma$ of the mean magnitude.

§Number of observations.

‖Observer's code: OKU (Osaka Kyoiku U.), hho (Kanata, Hiroshima U.), Ioh (H. Itoh), KU1 (Kyoto U., campus obs.), ISH (Murikabushi, Ishigakijima Astronomical Obs.).

#Filter. "C" means no filter (clear).

**Table E3.** Times of superhump maxima in ASASSN-18aan.

| $E$ | max* | error | $O-C$† | $N$‡ |
|---|---|---|---|---|
| 0 | 58458.3911 | 0.0005 | -0.0938 | 170 |
| 1 | 58458.5554 | 0.0004 | -0.0874 | 289 |
| 6 | 58459.3836 | 0.0006 | -0.0487 | 148 |
| 7 | 58459.5437 | 0.0006 | -0.0465 | 85 |
| 10 | 58460.0611 | 0.0010 | -0.0028 | 31 |
| 16 | 58461.0111 | 0.0007 | -0.0002 | 137 |
| 17 | 58461.1779 | 0.0015 | 0.0087 | 132 |
| 18 | 58461.3274 | 0.0003 | 0.0003 | 224 |
| 19 | 58461.4848 | 0.0006 | -0.0002 | 127 |
| 20 | 58461.6464 | 0.0012 | 0.0035 | 66 |
| 22 | 58461.9705 | 0.0008 | 0.0118 | 190 |
| 23 | 58462.1268 | 0.0015 | 0.0102 | 72 |
| 30 | 58463.2352 | 0.0006 | 0.0133 | 833 |
| 31 | 58463.3980 | 0.0008 | 0.0182 | 118 |
| 32 | 58463.5470 | 0.0006 | 0.0093 | 119 |
| 41 | 58464.9680 | 0.0007 | 0.0092 | 200 |
| 42 | 58465.1313 | 0.0012 | 0.0146 | 44 |
| 48 | 58466.0768 | 0.0015 | 0.0127 | 139 |
| 50 | 58466.3930 | 0.0007 | 0.0131 | 114 |
| 54 | 58467.0636 | 0.0013 | 0.0521 | 234 |
| 56 | 58467.3590 | 0.0011 | 0.0317 | 65 |
| 60 | 58467.9643 | 0.0026 | 0.0054 | 329 |
| 68 | 58469.2421 | 0.0036 | 0.0200 | 126 |
| 82 | 58471.3935 | 0.0051 | -0.0392 | 103 |
| 83 | 58471.5495 | 0.0034 | -0.0411 | 176 |
| 86 | 58471.9996 | 0.0032 | -0.0647 | 127 |
| 88 | 58472.2854 | 0.0011 | -0.0947 | 32 |

*BJD−2400000.

†$C$ = 2458461.485+0.1579$E$.

‡Number of points used to determine the maximum.
